# Supplementary material for: ExceLint: Automatically Finding Spreadsheet Formula Errors
Source: arXiv:1901.11100 source file (2019-01-30)
Supplement: Supplementary file 1 [file appendix.tex]

%\begin{figure*}[H]
%\centering
%   \begin{subfigure}[b]{0.3\textwidth}
%   \includegraphics[width=0.8\textwidth]{images/ex_precision_plot.pdf}
%   \caption{}
%   \label{fig:ExPrecisionPlot}} 
%\end{subfigure}
%\begin{subfigure}[b]{0.3\textwidth}
%   \includegraphics[width=0.8\textwidth]{images/c_precision_plot.pdf}
%   \caption{}
%   \label{fig:CPrecisionPlot}
%\end{subfigure}
%\caption{(a) \excelint's precision is generally high across the \custodes benchmark suite.  In most cases, adjusting the precision based on the expected number of cells flagged by a random flagger has little effect. (b) \custodes precision is generally lower than \excelint's.  All results are sorted by adjusted precision (see Section~\ref{sec:rq2}).}
%\end{figure*}
